# Supplementary material for: Exploration of new experimental strategies for the detection of ultralight dark matter : laboratory searches on ground and in space
Source: arXiv:2411.14128 source file (2024-11-21)
Supplement: Supplementary file 1 [file appendix00.tex]

For a given signal in time domain $s(t)$, we can define its discrete Fourier transform as 
\begin{align}
    \Tilde{s}_k(f) = \sum_{m=0}^{N-1} s_m e^{-\frac{2\pi i m k}{N}}
\end{align}
where $N$ is the number of measurements. 
The signal PSD is defined as the square modulus of $\Tilde{s}_k$ divided by the frequency bandwidth of the data taking, defined as $df=f_s/N$, where $f_s$ is the sampling frequency.
If we further assume that the measurement is continuous during the whole time of observation, i.e $T_\mathrm{int} = N \Delta t$, where $\Delta t=1/f_s$ is the time between measurements, we have 
\begin{align}
    S_s(f) &= |\Tilde{s}_k(f)|^2 T_\mathrm{int}
    \label{sig_PSD_no_coherence}
\end{align}
Then, putting everything together, the signal is found to be 
\begin{align}
    \Tilde{s}_k(f) &= \sqrt{\mathrm{SNR}}\sqrt{\frac{S_n(f)}{T_\mathrm{int}}}
\end{align}

\jg{think about that}
Eq.~\eqref{sig_PSD_no_coherence} works only for perfectly coherent signal, or in other words when $T_\mathrm{int} < \tau(\omega_\mathrm{DM})$ in our model. In that case, the signal is monochromatic and the PSD is simply a spike in frequency domain.

When $T_\mathrm{int} > \tau(\omega_\mathrm{DM})$, the signal PSD has a finite width which is directly coming from the DM velocity dispersion described in Section.~\ref{sec:coherence_DM}. 
For the estimation of the sensitivity in such scenario, we can use Bartlett's method \cite{Budker14} whose principle is quite straightforward. The idea is to cut the signal in $T_B$ parts with duration $\tau_B$ such that $\tau_B < \tau(\omega_\mathrm{DM})$. Then, in those restricted time regions, the signal is expected to be monochromatic and the above method can be applied to estimate those partial PSD. The total PSD over the full time $T_\mathrm{int}$ is found by averaging all the partial ones, which as a consequence decreases the noise PSD by a factor $\sqrt{T_\mathrm{int}/\tau_B}$.
In the limit where $\tau_B \rightarrow \tau(\omega_\mathrm{DM})$, the sensitivity of such experiment becomes 
\begin{align}
    \Tilde{s}_k(f) &= \sqrt{\mathrm{SNR}}\sqrt{\frac{S_n(f)}{\sqrt{T_\mathrm{int}\tau(\omega_\mathrm{DM})}}}
\end{align}
